# Supplementary material for: Laser pulse driven control of charge and spin order in the two-dimensional Kondo lattice
Source: arXiv:2002.03023 ancillary file (2020-02-07)
Supplement: Supplementary file 1 [file Supplemental.pdf]

# Supplementary Material for "Laser pulse driven control of charge and spin order in the two-dimensional Kondo lattice"

Benedikt Fauseweh[1,*] and Jian-Xin Zhu[1,2,†]

[1] Theoretical Division, Los Alamos National Laboratory, Los Alamos, New Mexico 87545, USA
[2] Center for Integrated Nanotechnologies, Los Alamos National Laboratory, Los Alamos, New Mexico 87545, USA

(Dated: February 6, 2020)

## TIME-DEPENDENT VARIATIONAL MONTE CARLO

The concept of time-dependent Variational Monte Carlo (tVMC) was introduced by Carleo and co-workers for bosonic systems in [1, 2] and extended to strongly correlated fermionic systems by the Imada group in [3]. It has also been applied to spin systems [4, 5]. Recent progress focuses on advancing the efficency of tVMC by adapting neural networks as quantum states [6–10]. The starting point for tVMC is a variational wave function $|\Psi_{\boldsymbol{\alpha}}\rangle$ with complex variational parameters $\alpha$. The main aim of the variational wave function is to reduce the number of parameters to describe the physically relevant Hilbert space. To describe the time evolution of the variational parameters, the time-dependent variational principle is applied [11], which leads to

$$\frac{\mathrm{d}\boldsymbol{\alpha}}{\mathrm{d}t} = -i\,(S)^{-1}\,\mathbf{g} \qquad (1)$$

where the $S$ matrix and the vector $\mathbf{g}$ are given by

$$S_{kl} = \left\langle \mathcal{O}_k^\dagger \mathcal{O}_l \right\rangle - \left\langle \mathcal{O}_k^\dagger \right\rangle \left\langle \mathcal{O}_l \right\rangle \qquad (2)$$

$$g_l = \left\langle \mathcal{O}_l^\dagger H \right\rangle - \left\langle \mathcal{O}_l^\dagger \right\rangle \left\langle H \right\rangle . \qquad (3)$$

The derivative operators $\mathcal{O}_l$ describe the variational wave function upon changing the parameter $\alpha_l$. In an electron real space configuration basis $|x\rangle$ they are given by

$$O_l(x) = \frac{1}{\langle x|\Psi_{\boldsymbol{\alpha}}\rangle}\partial_{\alpha_l}\langle x|\Psi_{\boldsymbol{\alpha}}\rangle. \qquad (4)$$

In tVMC the expectation values appearing in $S$ and $\mathbf{g}$ are evaluted by sampling the configuration basis using the metropolis algorithm. In the following step the time evolution in (1) is solved. In our approach a 4th order Runge-Kutta algorithm with a stepwidth of $\delta_t = 0.01$ proved to produce stable dynamics. Note that the inversion of the $S$ matrix can be ill-defined, due to vanishing singular values. We therefore adapt the MINRES-QLP algorithm [12] to minimize the least square solution, effectively implementing the Penrose-Moore pseudoinverse.

## ENERGY DEPOSITION

During the pulse, energy is deposited in the system. Fig. 1 shows the energy per site as function of time.

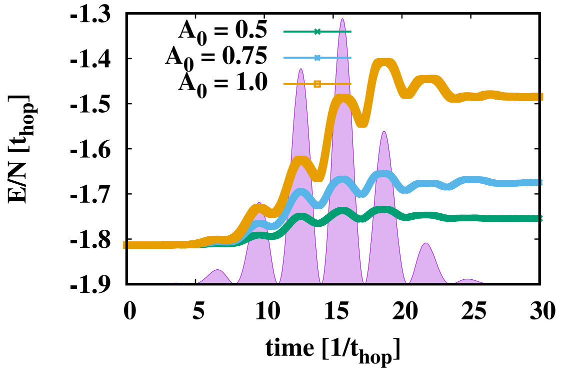


FIG. 1. Energy of the system as function of time. The shaded background is proportional to the squared pulse profile.

Notice that the total energy increase is proportional to the maximal pulse amplitude. Assuming a hopping of $t_{\mathrm{hop}} = 0.125$ eV and a lattice spacing of $a = 0.4656$ nm, as in the main text, the strongest pulse deposits an energy of $\propto 0.0028$ mJ/cm$^2$ on a single layer.

## SCALING OF THE CHARGE STRUCTURE FACTOR

In order to assess the electronic state of the system after the pump pulse, we investigate the small $\mathbf{q}$ behaviour of the charge structure factor $S_N(\mathbf{q})$. We assume, that a charge excitation can be described by the state

$$|\Psi_{\mathbf{q}}\rangle = n_{\mathbf{q}}\,|\Psi\rangle \ , \ n_{\mathbf{q}} = \sum_i e^{i\mathbf{q}\mathbf{r}_i} n_i \qquad (5)$$

where $|\Psi\rangle$ is the ground state wave function. Calculating the energy of such as state connects it directly to the charge structure factor [13], i.e. for $N_{\mathbf{q}} \propto |\mathbf{q}|$ there exist gapless charge modes; for $N_{\mathbf{q}} \propto |\mathbf{q}|^2$ the charge sector is gapped.

Fig. 2 shows the $\mathbf{q}$ dependence of $N_{\mathbf{q}}/|\mathbf{q}|$. This quantity is expected to scale to a constant for small $\mathbf{q}$ in presence of gapless excitations, while it scales as $|\mathbf{q}|$ for gapped systems. Although the scaling analysis is not perfect for the small system size, the transition from an insulator to a gapless system can described on a qualitative level.

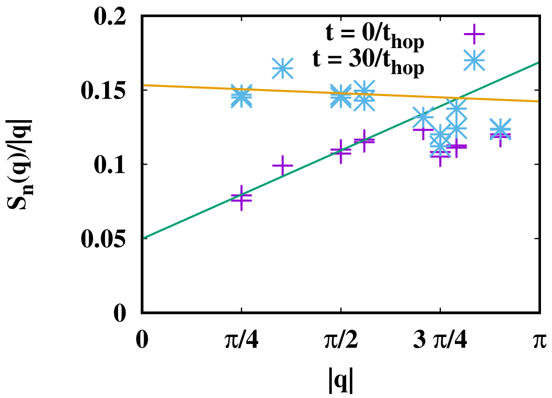


FIG. 2. Small $|\mathbf{q}|$ dependence of $N_{\mathbf{q}}/|\mathbf{q}|$ for the ground state at $t = 0/t_{\text{hop}}$ and for the post pulse state at $t = 30/t_{\text{hop}}$. Curves are fits to linear functions for $|\mathbf{q}| < 5/8\pi$.


* fauseweh@lanl.gov

† jxzhu@lanl.gov



[1] G. Carleo, F. Becca, M. Schiró, and M. Fabrizio, Scientific Reports **2**, 243 (2012).

[2] G. Carleo, F. Becca, L. Sanchez-Palencia, S. Sorella, and M. Fabrizio, Phys. Rev. A **89**, 031602 (2014).

[3] K. Ido, T. Ohgoe, and M. Imada, Phys. Rev. B **92**, 245106 (2015).

[4] L. Cevolani, G. Carleo, and L. Sanchez-Palencia, Phys. Rev. A **92**, 041603 (2015).

[5] G. Fabiani and J. H. Mentink, SciPost Phys. **7**, 4 (2019).

[6] G. Carleo and M. Troyer, Science **355**, 602 (2017).

[7] G. Carleo, Y. Nomura, and M. Imada, Nature Communications **9**, 5322 (2018).

[8] Y. Nomura, A. S. Darmawan, Y. Yamaji, and M. Imada, Phys. Rev. B **96**, 205152 (2017).

[9] M. Schmitt and M. Heyl, arXiv:1912.08828, (2019).

[10] I. Lpez-Gutirrez and C. B. Mendl, arXiv:1912.08831, (2019).

[11] J. Haegeman, T. J. Osborne, and F. Verstraete, Phys. Rev. B **88**, 075133 (2013).

[12] S.-C. T. Choi, C. C. Paige, and M. A. Saunders, SIAM Journal on Scientific Computing **33**, 1810 (2011).

[13] M. Capello, F. Becca, M. Fabrizio, S. Sorella, and E. Tosatti, Phys. Rev. Lett. **94**, 026406 (2005).
